# Supplementary material for: Stacking the spectra of eROSITA galaxy cluster data for searches of the 3.5keV line: Dark matter decay or charge exchange?
Source: arXiv:2401.00923 source file (2024-02-15)
Supplement: Supplementary file 1 [file Appendix.tex]

\appendix
